# Supplementary material for: Kinetics and Free Energy of Ligand Dissociation Using Weighted Ensemble Milestoning
Source: arXiv:2007.09325 ancillary file (2020-09-30)
Supplement: Supplementary file 1 [file Supp_info.pdf]

# Supplementary Material for: Kinetics and Free Energy of Ligand Dissociation Using Weighted Ensemble Milestoning

Dhiman Ray,<sup>†</sup> Trevor Gokey,<sup>†</sup> David Mobley,<sup>†,‡</sup> and Ioan Andricioaei<sup>\*,†,¶</sup>

<sup>†</sup> *Department of Chemistry, University of California Irvine, California 92697, USA*

<sup>‡</sup>*Department of Pharmaceutical Sciences, University of California Irvine, California 92697, USA*

<sup>¶</sup> *Department of Chemistry, Department of Physics and Astronomy, University of California Irvine, California 92697, USA*

E-mail: andricio@uci.edu.

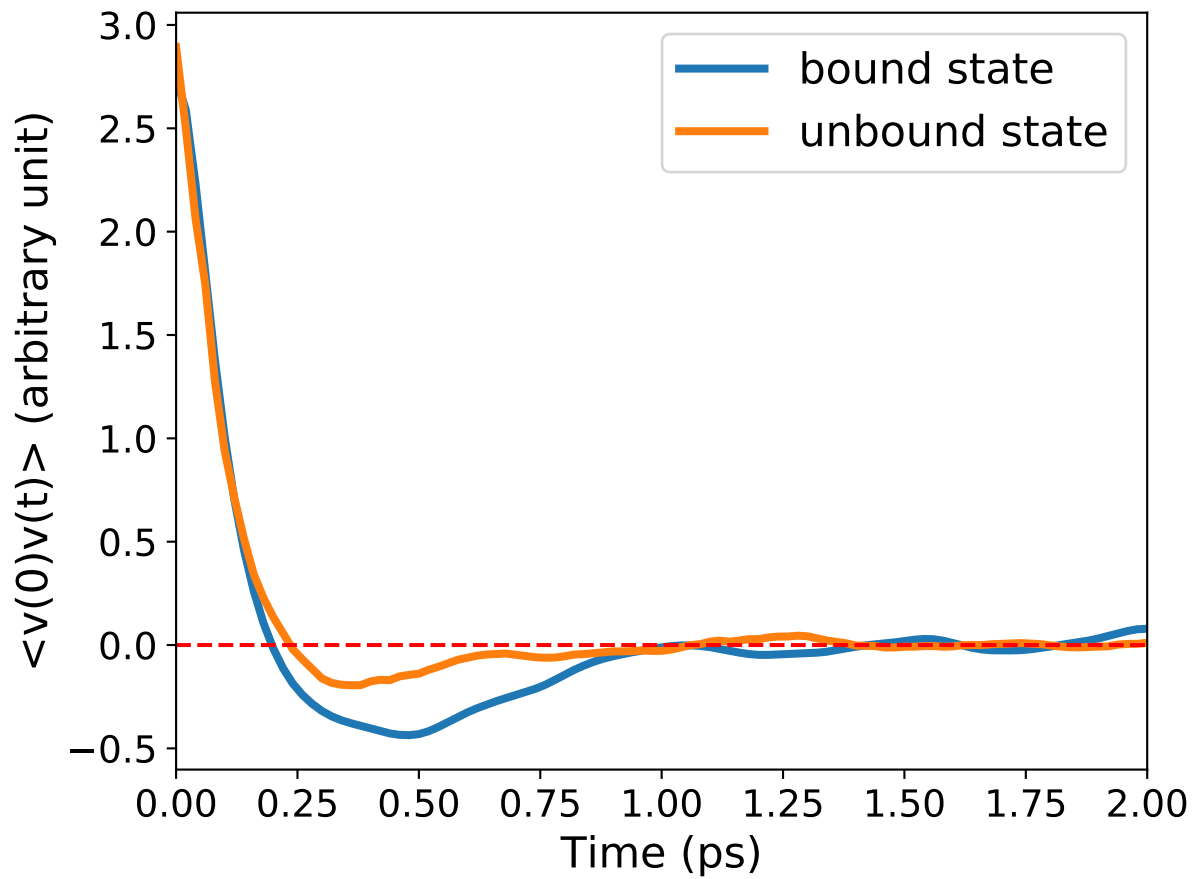

Figure S1: Velocity auto-correlation function of the reaction coordinate (protein-ligand distance) of the FKBP-BUT system computed from 1 ns equilibrium simulation in the bound and the unbound state. The correlation decays to zero in about 1 ps for bound state and 0.7 ps for the unbound state. Milestones are to be placed such a way that the fastest transition between them takes place at a longer time than the decorrelation timescale.

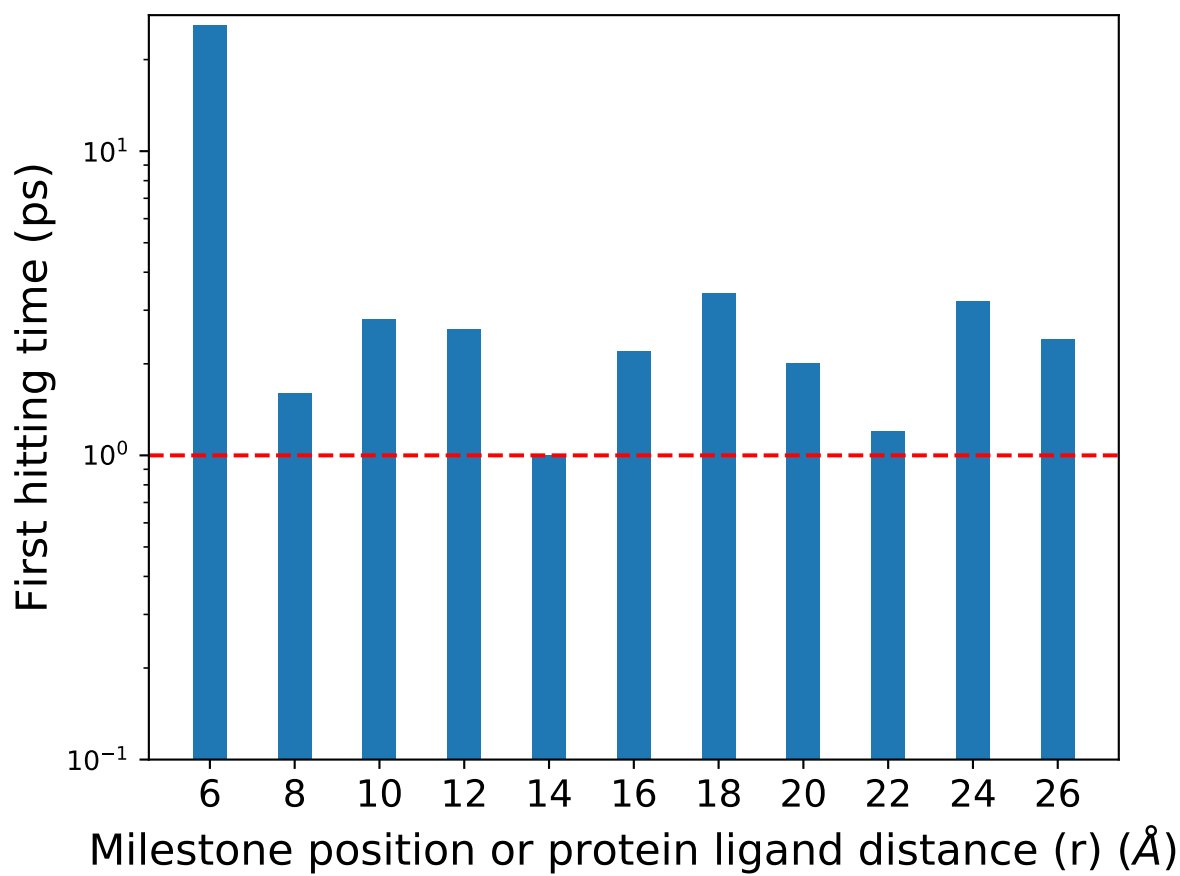

Figure S2: The first hitting time for the quickest trajectory starting from each individual milestone. Results are shown only for trial 1 of WEM RR simulation of FKBP-BUT system. The velocity decorrelation time for the reaction coordinate is  $\sim 1$  ps (Fig. S1), which is denoted as a red dashed line. The spacing between milestones are barely optimum as the first hitting time of the quickest trajectory is only slightly higher than the decorrelation time. Milestones which are more closely spaced will be prone to give spurious results.

**Well Tempered Metadynamics (WTMtd) simulation of FKBP+BTB system:**

Well Tempered Metadynamics (WTMtd) simulation was initiated from the equilibrated bound structure of the FKBP-BTB complex. Gaussian hills of  $\sigma = 1 \text{ \AA}$  were deposited at 1 ps interval along the protein ligand distance based reaction coordinate. The initial height of hills were 0.2 kcal/mol and a bias factor of 6.0 was employed. Converged PMF with  $< 1k_B T$  variation could be obtained from 100 ns WTMtd simulation. The simulation was performed for 120 ns and the last 20 ns of data was used for block averaging and error estimation. All other simulation parameters were identical to that described in the computational methods section of the original manuscript.

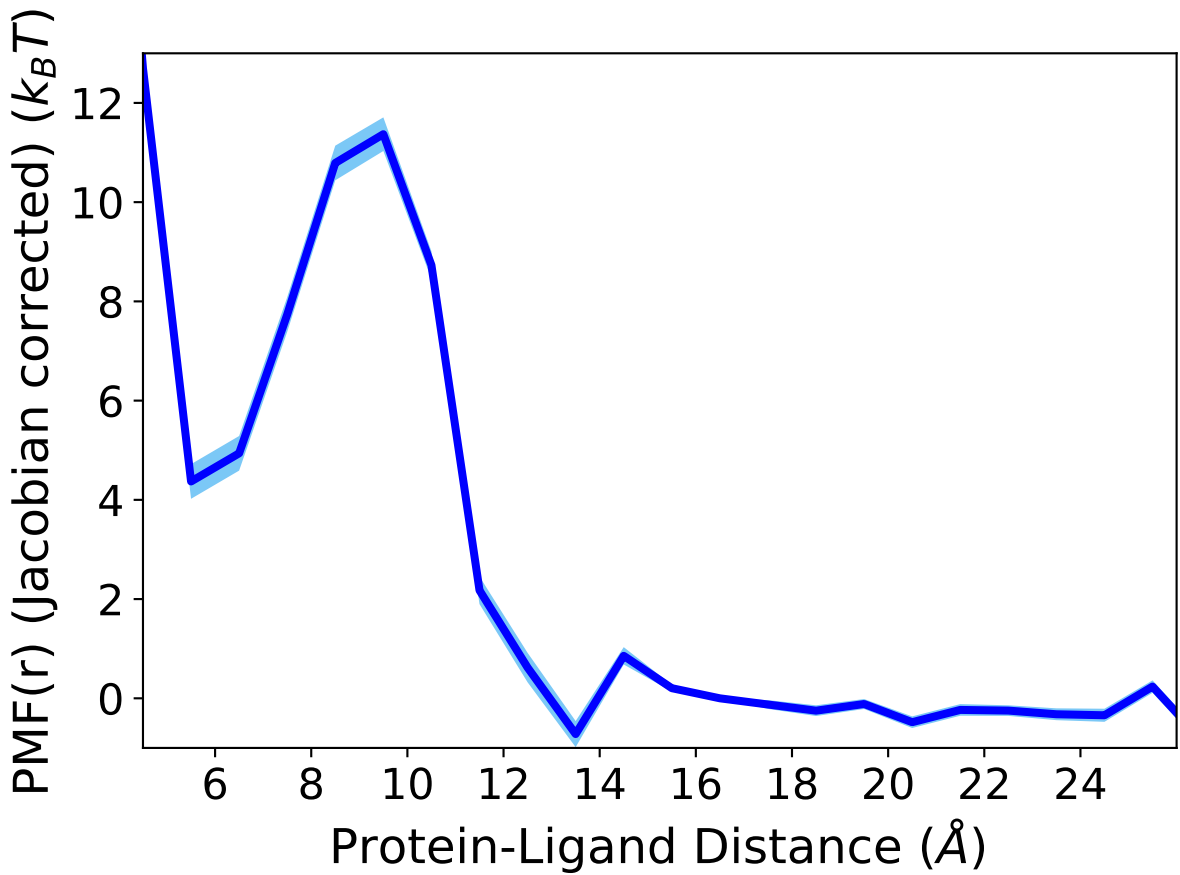

Figure S3: PMF of BTB ligand dissociation from FKBP protein computed using well tempered metadynamics simulation. Error bars are 95% confidence intervals obtained from 10 PMF's calculated at 2 ns interval for the last 20 ns of the simulation.

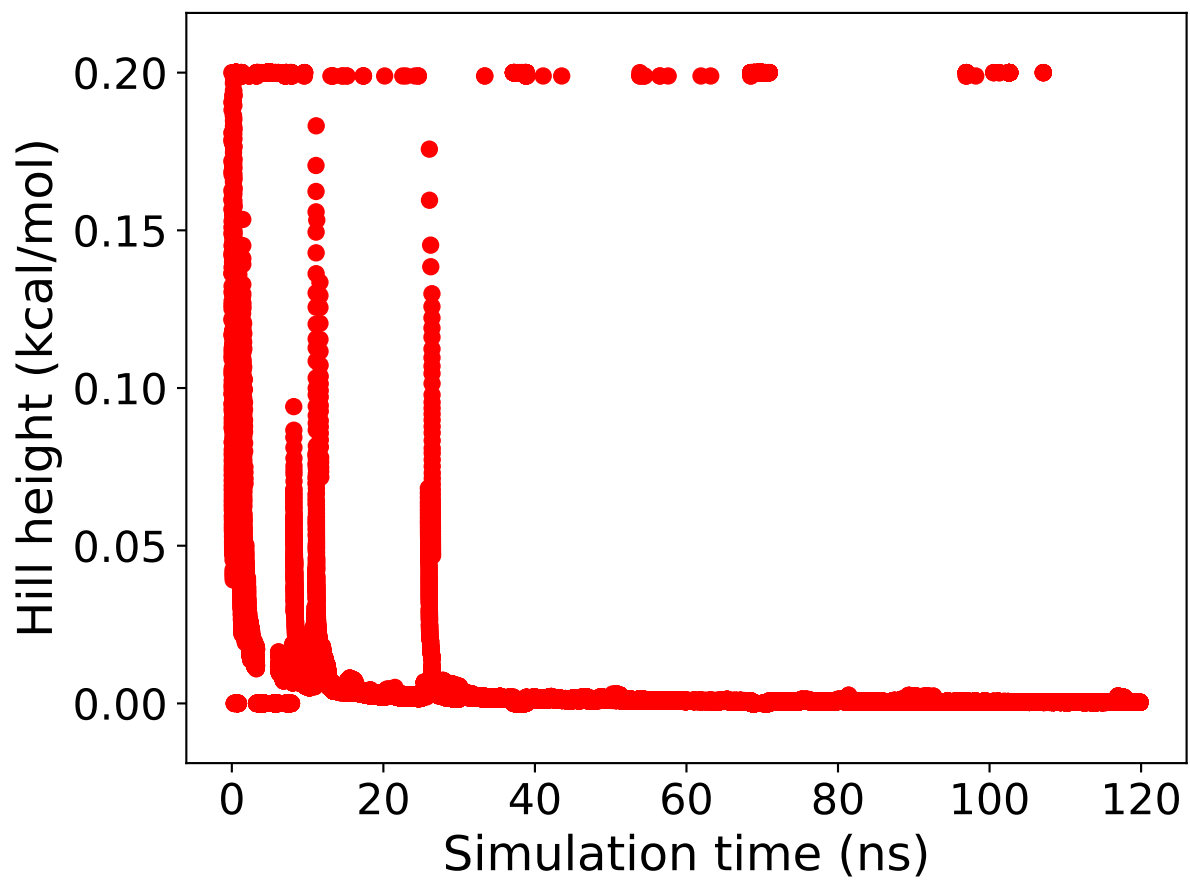

Figure S4: Convergence check of the WTMtD simulation by monitoring the time evolution of the bias or the Gaussian hill heights which approaches zero. It remains fairly unchanged towards the end of the simulation.

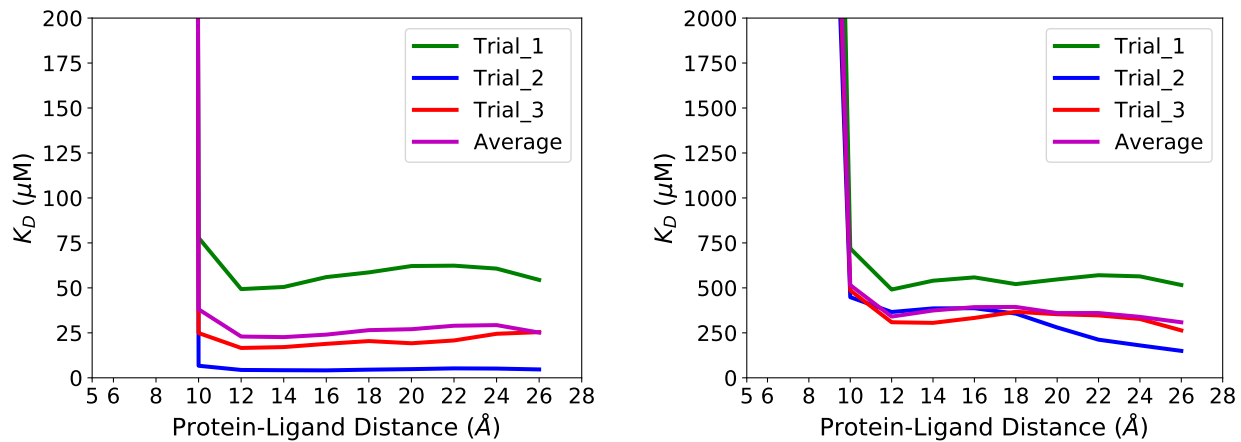

Figure S5:  $K_D$  along the center of mass distance between FKBP protein and BUT ligand: (left) using normal WEM calculation and (right) using harmonic constrain release to generate multiple initial condition per milestone.

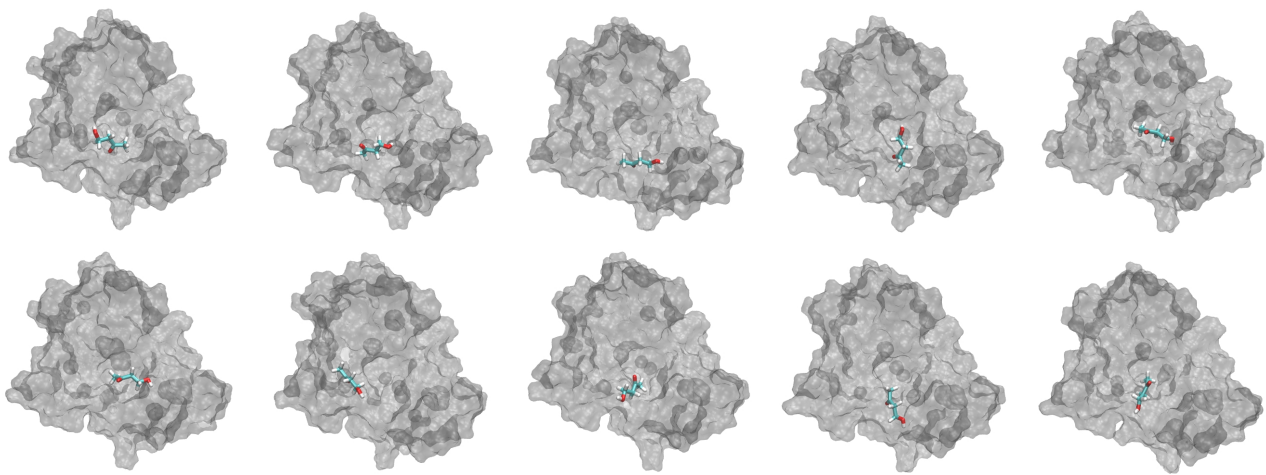

Figure S6: The 10 starting points sampled from harmonically restrained weighted ensemble simulation for milestone at  $r = 16$  Å.

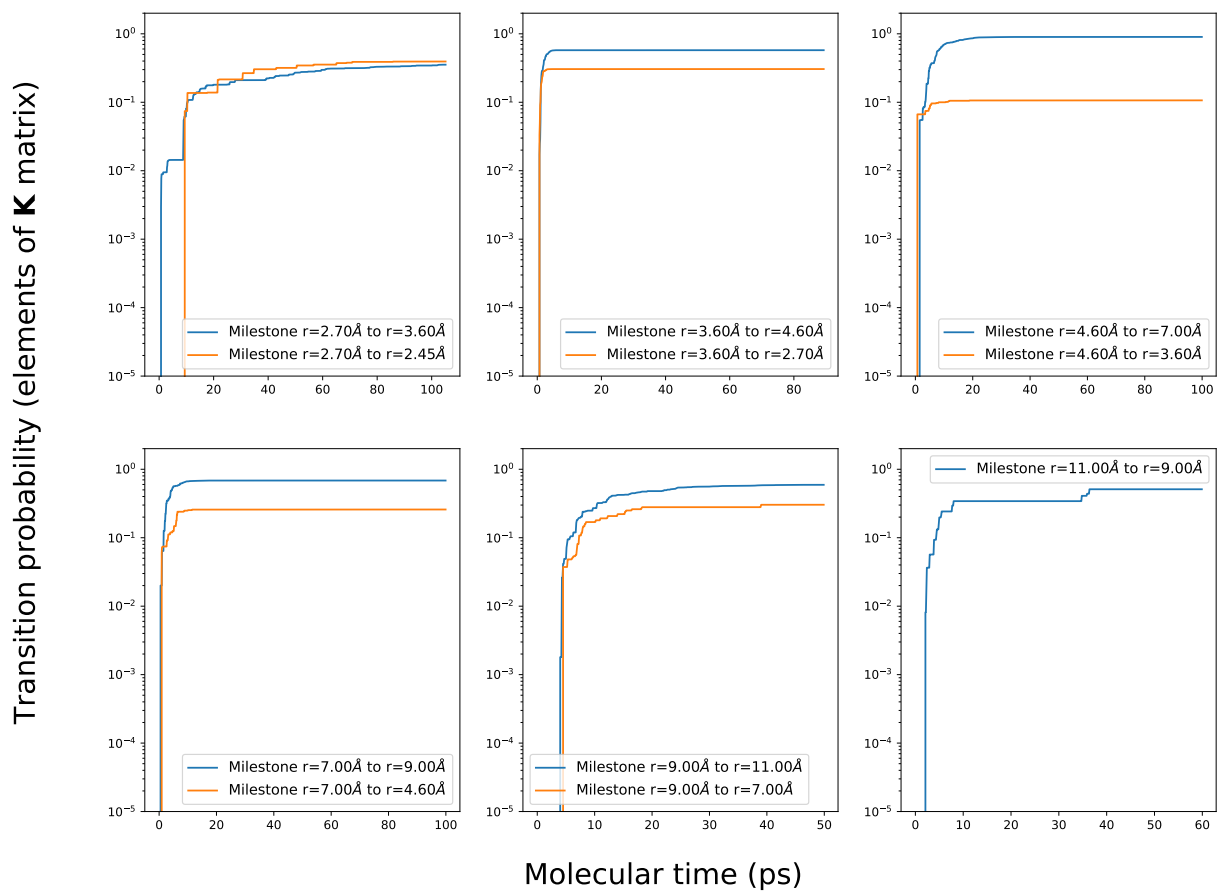

Figure S7: Convergence of transition probability matrix elements  $K_{ij}$  for the trial 1 of WEM simulation of Na<sup>+</sup>/Cl<sup>-</sup> ion pair. Definition of molecular time is according to Adhikari et al.<sup>1</sup>

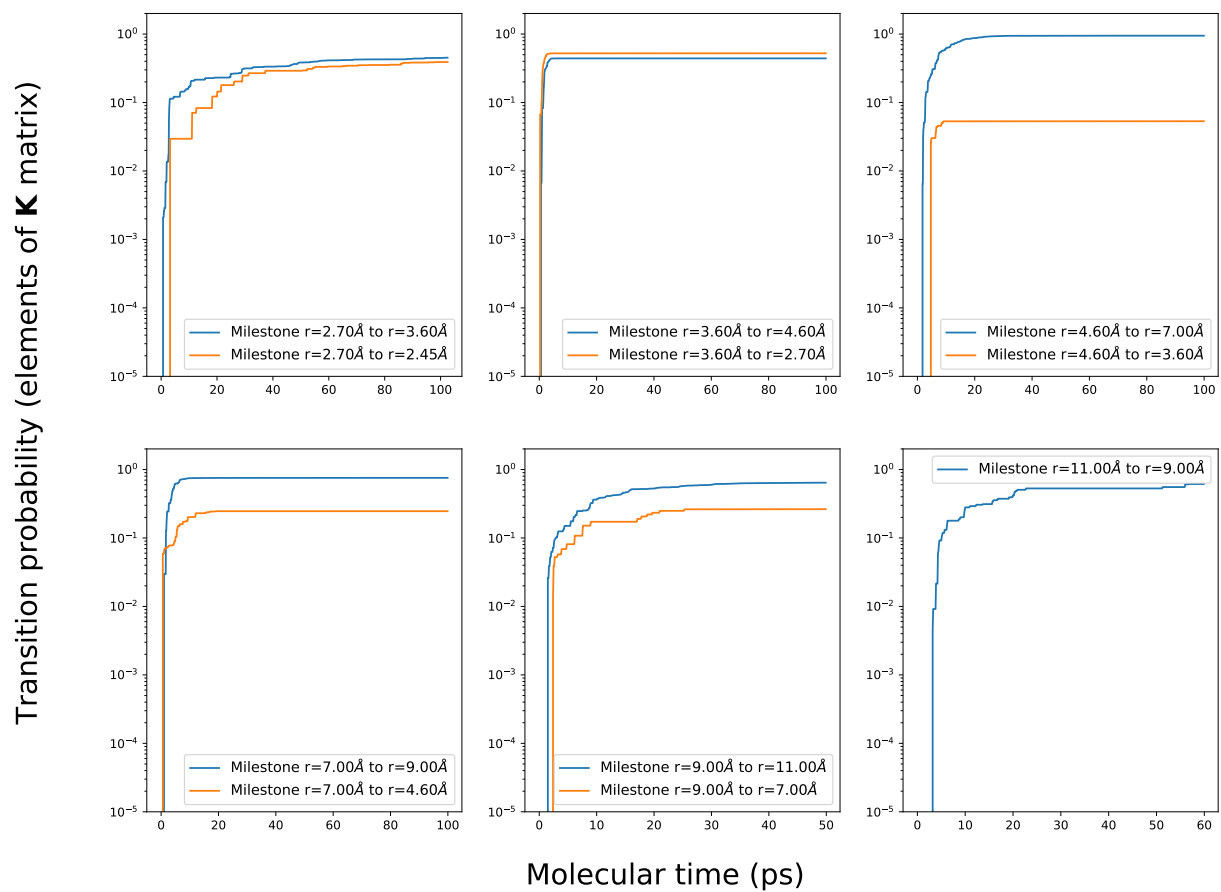

Figure S8: Same as Figure S7 but for trial 2

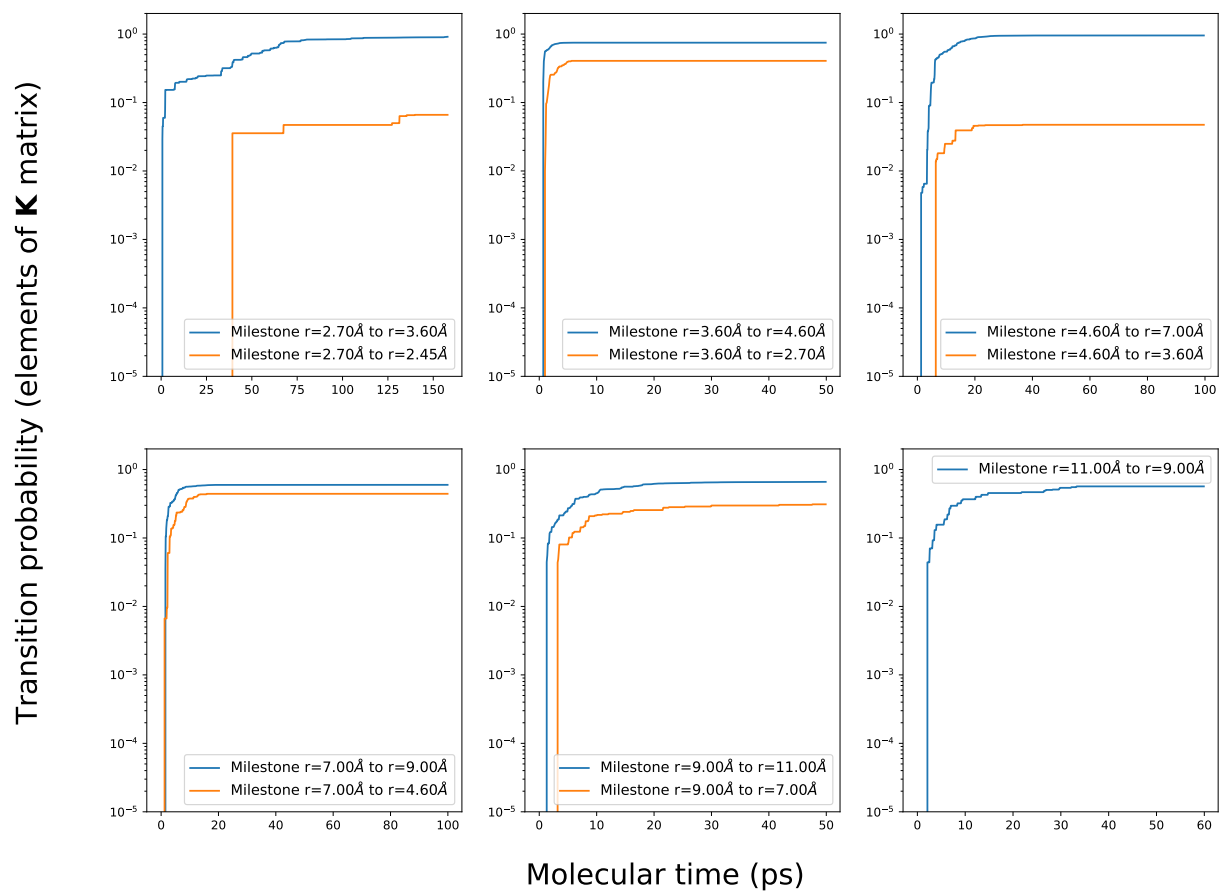

Figure S9: Same as Figure S7 but for trial 3

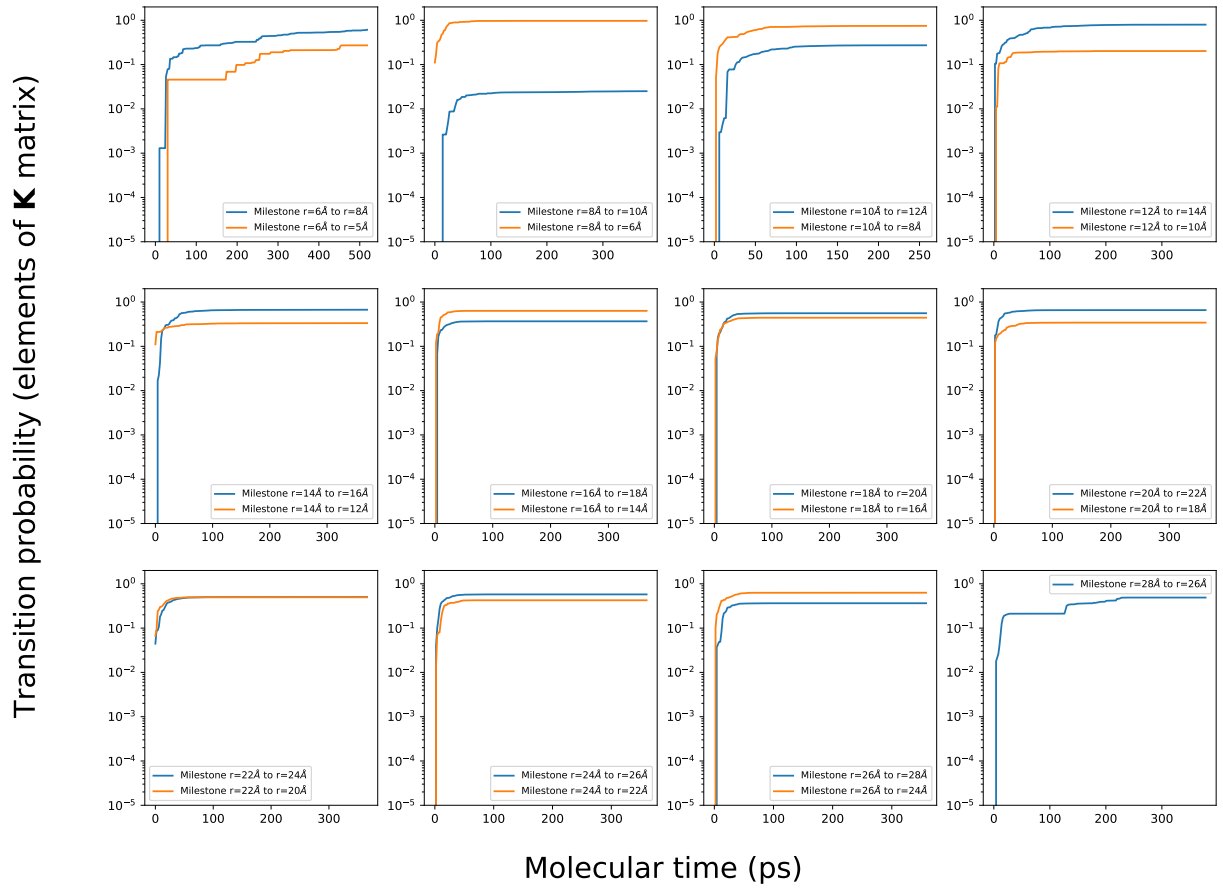

Figure S10: Convergence of transition probability matrix elements  $K_{ij}$  for the trial 1 of WEM-RR simulation of FKBP+BTB system. Definition of molecular time is according to Adhikari et al.<sup>1</sup>

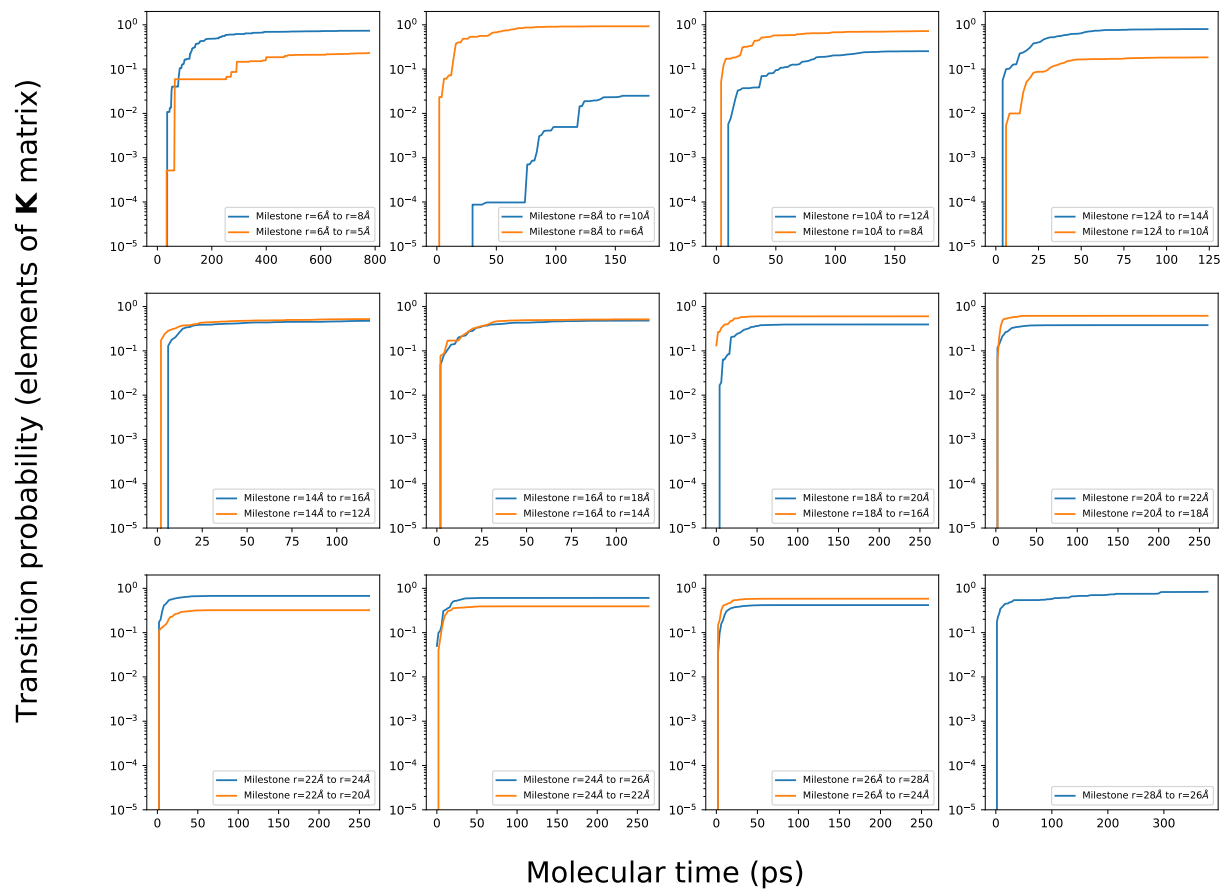

Figure S11: Same as Figure S10 but for trial 2

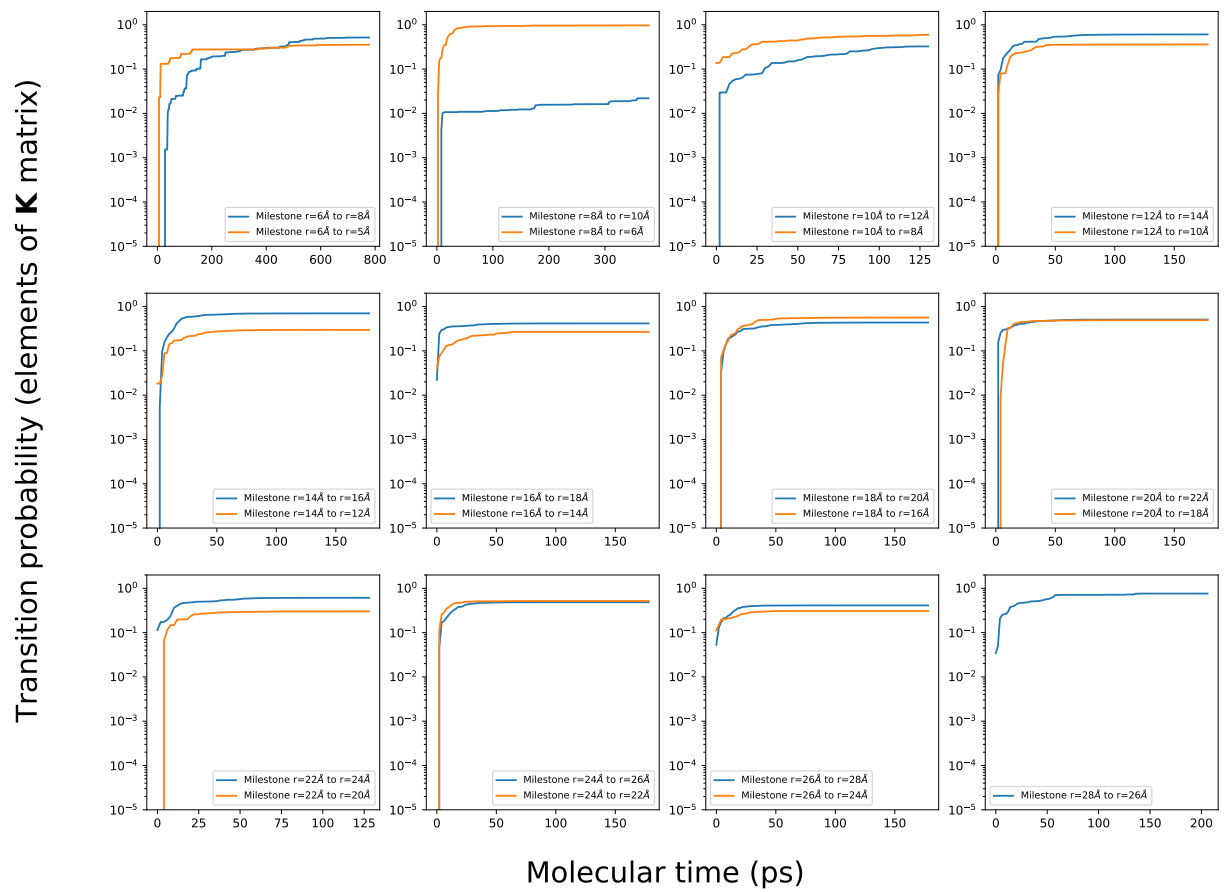

Figure S12: Same as Figure S10 but for trial 3

## References

- (1) Adhikari, U.; Mostofian, B.; Copperman, J.; Subramanian, S. R.; Petersen, A. A.; Zuckerman, D. M. Computational Estimation of Microsecond to Second Atomistic Folding Times. *Journal of the American Chemical Society* **2019**, *141*, 6519–6526.
